# Supplementary material for: Machine Translation System Selection from Bandit Feedback
Source: arXiv:2002.09646 source file (2020-09-02)
Supplement: Supplementary file 1 [file 07_appendix.tex]

\appendix

\section{Supplemental Material}
\label{sec:supplemental}

\includegraphics[scale=0.3]{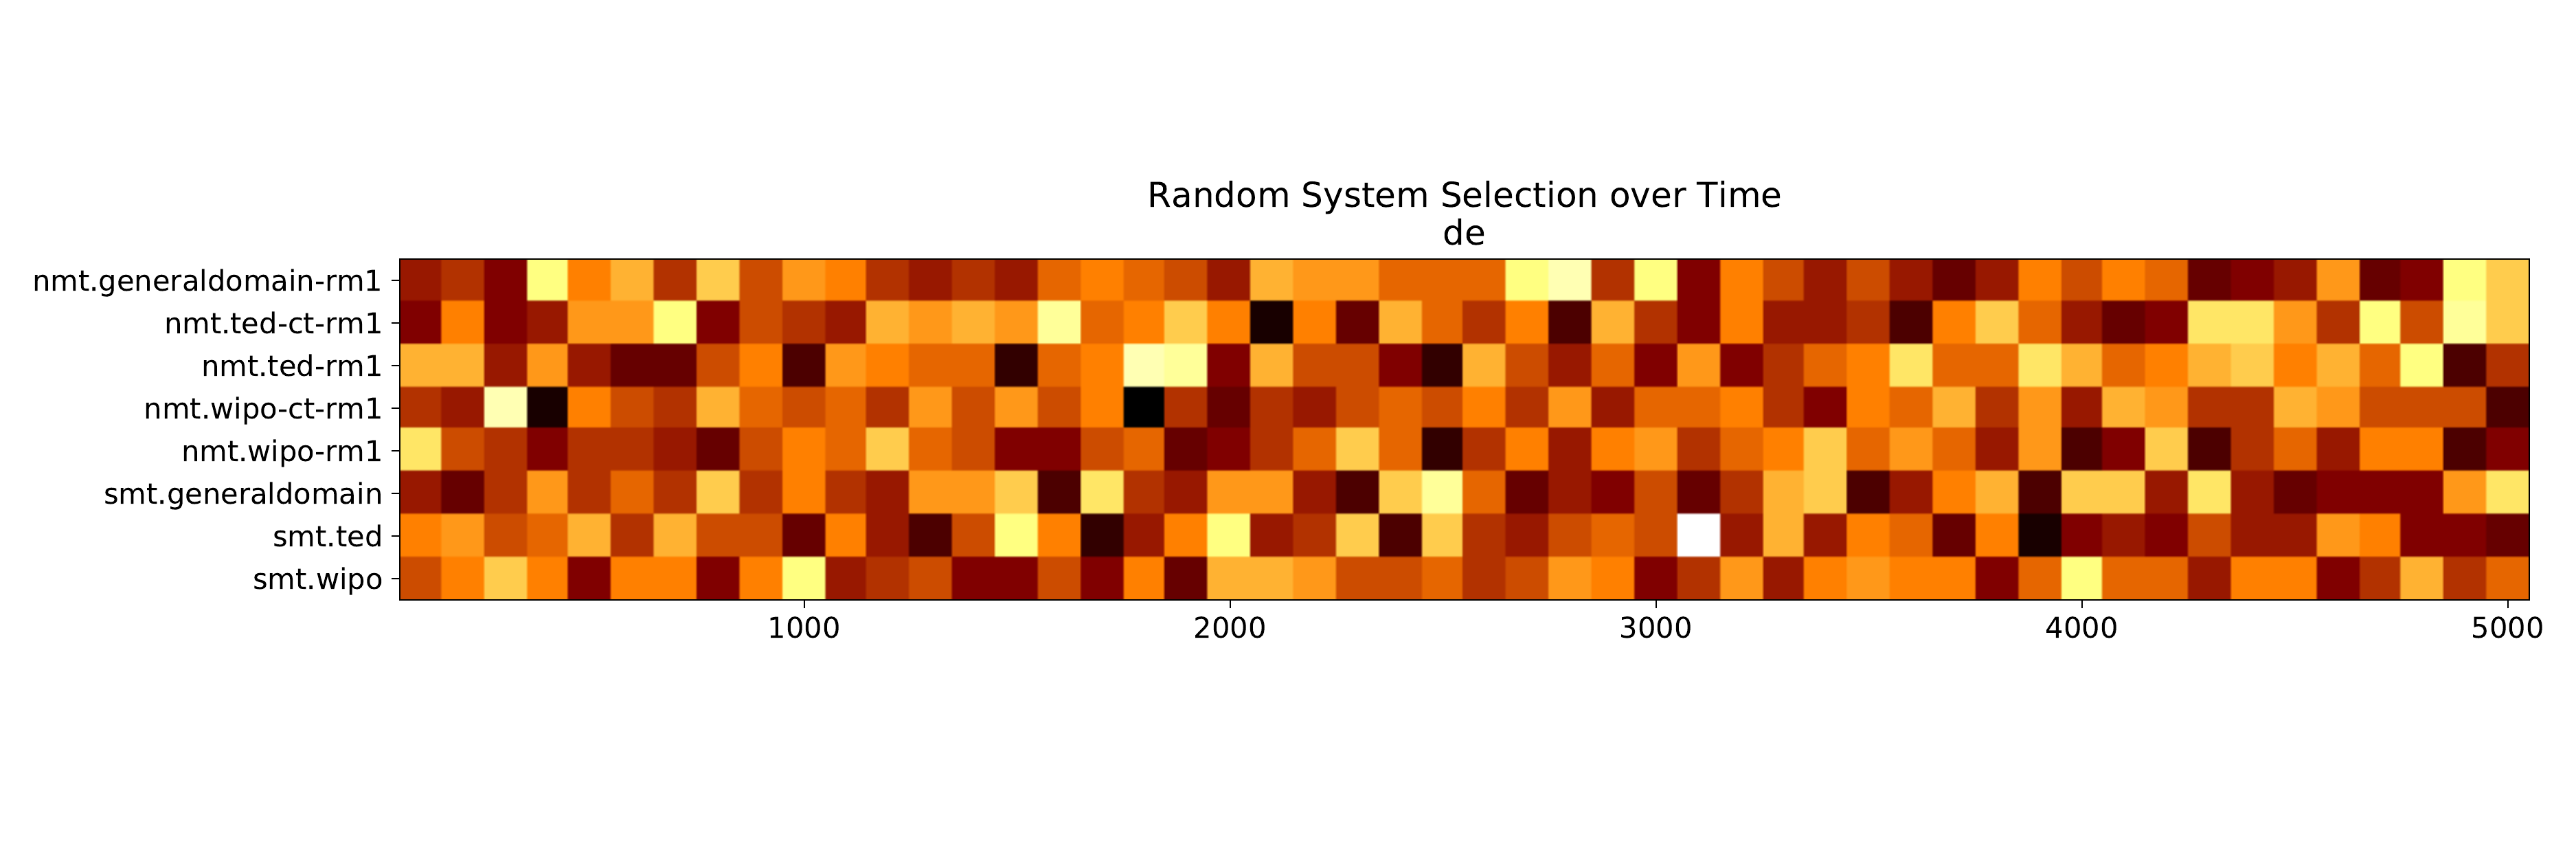}

\includegraphics[scale=0.5]{images/tmp/de__g1000_w1000_t1000_g1000_w500_t500_plot.pdf}

\clearpage
